# Supplementary material for: BART with Targeted Smoothing: An analysis of patient-specific stillbirth risk
Source: arXiv:1805.07656 source file (2019-06-03)
Supplement: Supplementary file 1 [file 07-supplementary-materials.tex]

%!TEX root = ../tsbart-paper.tex

The \methN{} R package \textbf{tsbart} can be found at \url{https://github.com/jestarling/tsbart}.
